# Supplementary material for: ProxyPrompt: Securing System Prompts against Prompt Extraction Attacks
Source: arXiv:2505.11459 source file (2026-04-29)
Supplement: Supplementary file 2 [file 20_attack_query.tex]

Our evaluation uses a comprehensive set of 193 attack queries aggregated from four recent studies.  
This collection is intentionally diverse, spanning a wide range of prompt-extraction strategies, linguistic variants, and obfuscation styles. Below we provide the full breakdown:

\begin{itemize}
    \item \textbf{123 queries from \citet{guess_prompt}}:  
    These include instructions that explicitly or implicitly attempt to bypass system-level safeguards, such as asking the model to ignore prior instructions, restate internal rules, or transform its output (e.g., through reversible ciphers or formatting constraints).

    \item \textbf{4 optimized extraction queries from \citet{hui2024pleak}}:  
    These were designed specifically to extract system prompts from Poe-based LLM applications~\citep{poe} and are closely aligned with our \textsc{Roles} task setting. They were obtained using iterative query optimization through shadow models.

    \item \textbf{44 queries from \citet{wang2024raccoon}}:  
    These cover 14 attack categories from the Raccoon benchmark, including multilingual attacks and prompt injections hidden inside Python dictionaries.

    \item \textbf{22 queries from \citet{why_leaked}}:  
    These include both explicit and implicit instructions to extract system prompts.
\end{itemize}

This combination ensures high attack diversity, including adversarial queries that differ in surface form, linguistic structure, intent masking, and encoding.
