# Supplementary material for: ProxyPrompt: Securing System Prompts against Prompt Extraction Attacks
Source: arXiv:2505.11459 source file (2026-04-29)
Supplement: Supplementary file 3 [file 04_ablation_study.tex]

We detail the results of our ablation study in~\Cref{tab:ablation} as introduced in the analysis of~\Cref{subsec:experimental_results}, which examines the impact of removing the extraction prevention loss $\mathcal{L}\Big(f_{\tilde{\phi}_P||\phi_{P'}}(\phi_{Q'}), \tilde{P} \Big)$ from our joint optimization objective (\Cref{eq:joint_loss}). The study demonstrates the importance of the joint optimization in achieving robust defense against prompt extraction attacks.

\begin{table*}[h!]
\caption{Effect of removing extraction prevention loss, i.e. $\Ls(R', \tilde{P})$, on prompt extraction success and utility preservation across different tasks and model configurations.}
\label{tab:ablation}
\vskip 0.15in
\begin{center}
{\fontsize{6.8}{10}\selectfont
\setlength{\tabcolsep}{2.1pt}
\begin{tabular}{llccccccccccccccccccccccc}
\toprule
\textbf{Victim} & \textbf{Defense} & \multicolumn{4}{c}{\textbf{GSM8K}} & \multicolumn{4}{c}{\textbf{Roles}} & \multicolumn{4}{c}{\textbf{CoLA}} & \multicolumn{4}{c}{\textbf{SST-2}} & \multicolumn{4}{c}{\textbf{QNLI}} \\
\cmidrule(lr){3-6} \cmidrule(lr){7-10} \cmidrule(lr){11-14} \cmidrule(lr){15-18} \cmidrule(lr){19-22}
 & & UR & AM & SM & MS & UR & AM & SM & MS & UR & AM & SM & MS & UR & AM & SM & MS & UR & AM & SM & MS \\
\midrule
L-70B & \textsc{Ours}                            & \textbf{0.99} & \textbf{0.00} & \textbf{0.00} & \textbf{0.17} & \textbf{1.00} & \textbf{0.00} & \textbf{0.00} & \textbf{0.27} & 0.98 & \textbf{0.00} & \textbf{0.00} & \textbf{0.42} & \textbf{1.00} & \textbf{0.00} & \textbf{0.25} & \textbf{0.52} & \textbf{0.99} & \textbf{0.00} & \textbf{0.00} & \textbf{0.38} \\
& \textsc{w/o} $\Ls(R', \tilde{P})$  & 0.98 & \textbf{0.00} & \textbf{0.00} & 0.20 & \textbf{1.00} & \textbf{0.00} & \textbf{0.00} & 0.40 & \textbf{1.00} & \textbf{0.00} & 0.25 & 0.57 & 0.99 & \textbf{0.00} & 0.55 & 0.69 & 0.97 & \textbf{0.00} & 0.05 & 0.45 \\
\midrule
L-8B  & \textsc{Ours}                            & 0.99 & \textbf{0.00} & \textbf{0.00} & \textbf{0.18} & \textbf{1.00} & \textbf{0.00} & \textbf{0.00} & 0.31 & \textbf{1.01} & \textbf{0.00} & \textbf{0.05} & \textbf{0.40} & \textbf{1.00} & \textbf{0.00} & \textbf{0.10} & \textbf{0.53} & 0.94 & \textbf{0.00} & \textbf{0.05} & \textbf{0.38} \\
 & \textsc{w/o} $\Ls(R', \tilde{P})$ & \textbf{1.00} & \textbf{0.00} & 0.13 & 0.23 & \textbf{1.00} & \textbf{0.00} & \textbf{0.00} & \textbf{0.29} & \textbf{1.01} & \textbf{0.00} & 0.25 & 0.54 & \textbf{1.00} & \textbf{0.00} & 0.20 & 0.69 & \textbf{0.99} & \textbf{0.00} & 0.15 & 0.49 \\
\midrule
P-3.8B  & \textsc{Ours}                        & 0.99 & \textbf{0.00} & \textbf{0.00} & \textbf{0.18} & \textbf{1.00} & \textbf{0.00} & \textbf{0.00} & \textbf{0.22} & 0.93 & \textbf{0.00} & \textbf{0.00} & \textbf{0.37} & 0.97 & \textbf{0.00} & \textbf{0.25} & \textbf{0.50} & 0.95 & \textbf{0.00} & \textbf{0.00} & \textbf{0.49} \\
 & \textsc{w/o} $\Ls(R', \tilde{P})$ & \textbf{1.00} & \textbf{0.00} & 0.25 & 0.36 & \textbf{1.00} & \textbf{0.00} & \textbf{0.00} & 0.34 & \textbf{0.98} & \textbf{0.00} & 0.35 & 0.61 & \textbf{1.00} & \textbf{0.00} & 0.55 & 0.71 & \textbf{0.98} & \textbf{0.00} & \textbf{0.00} & 0.59 \\
\bottomrule
\end{tabular}
}
\end{center}
\end{table*}
