# Supplementary material for: ProxyPrompt: Securing System Prompts against Prompt Extraction Attacks
Source: arXiv:2505.11459 source file (2026-04-29)
Supplement: Supplementary file 5 [file 07_img_generator.tex]

% We provide the system prompt of Image Generator~\citep{img_generator} in~\Cref{tab:task_prompts_img_generator}, along with an example of relevant query and their corresponding responses. Specifically, secured response $\tilde{R}$ is the response after applying our ProxyPrompt.
% Our secured response $\tilde{R}$ is exactly the same as the predicted response $\hat{R}$, and has minor difference with the desired response $R$, which is generated with a temperature of 1 to encourage diversity.
% We also demonstrate examples of attack queries and their corresponding responses as the extracted prompt $G=f_{\tilde{\phi}_P}(A)$ after applying ProxyPrompt in~\Cref{tab:task_prompts_img_generator}.

\begin{figure}[h]
    \centering
    \includegraphics[width=1.0 \textwidth]{figs/img_generator_utility.png}
    \caption{Given a relevant query for image generation, ProxyPrompt for Image Generator, produces the same response as the original system prompt, confirming that utility is preserved.}
    \label{fig:img_generator_utility}
\end{figure}
